# Supplementary material for: Detecting Parkinson's Disease From an Online Speech-task
Source: arXiv:2009.01231 source file (2020-12-15)
Supplement: Supplementary file 1 [file supplementary_materials.tex]

\subsection{Predicting PD from Home-environment data only}

\begin{table*}
  \caption{The performance of various machine learning algorithms using  the Standard-features and Embedding-features on the Home-environment data as the test set. The models were trained on both Home-environment and Lab-environment data, but the performance metrics are calculated  on the Home-environment data only. The models using Standard-features perform better than their counterparts using Embedding-features in terms of both Binary Accuracy and AUC. \textcolor{orange}{Although the model's perform similarly in using the Standard-features, XGBoost outperforms others by considering both the AUC and Accuracy metrics}. However, the performance is slightly \st{lower}\textcolor{green}{worse} than the XGBoost model that uses both Home and Lab environment data in the test set: 0.0123 \textcolor{green}{decrease} in AUC and 0.004 \textcolor{green}{decrease} in Accuracy }
  \label{tab:res_super_park_not_in_test}
  \centering

\begin{tabular}{|l|l|l|l|l|l|l|l|l|}
\hline
Algorithm & \multicolumn{2}{|l|}{Standard-features} & \multicolumn{2}{|l|}{Embedding-features} \\ \hline
  & AUC  & Accuracy & AUC  & Accuracy \\\hline
 SVM & 0.7368  & 0.7336 & 0.7265  & 0.6964 \\
\hline
Random Forest  & 0.7317  & 0.7173 & 0.7194  & 0.7143 \\
\hline

LightGBM  & 0.7317 & 
0.7173 & 0.7327 & 0.6979 \\
\hline
XGBoost & \textbf{0.7379}  & \textbf{0.7366} & 0.7165  & 0.6949 \\
\hline

\end{tabular}

\end{table*}

% \begin{table*}
%   \caption{Results without SUPER-PARK in test-set}
%   \label{tab:res_super_park_not_in_test}
%   \centering
% \resizebox{\textwidth}{!}{
% \begin{tabular}{|l|l|l|l|l|l|l|l|l|l|l|l|l|l|l|}
% \hline
% Algorithm & \multicolumn{3}{|l|}{PRAAT} & \multicolumn{3}{|l|}{Max Little} & \multicolumn{3}{|l|}{Max Little + PRAAT} & \multicolumn{3}{|l|}{PASE} \\ \hline
%  & AUC & F1 & Acc. & AUC & F1 & Acc. & AUC & F1 & Acc. & AUC & F1 & Acc. \\\hline
% LightGBM & 0.6141 & 0.4449 & 0.625 & 0.7489 & 0.5548 & 0.7158 & 0.7317 & 0.5548 &
% 0.7173 & 0.7327 & 0.5522 & 0.6979 \\
% \hline
% XGBoost & 0.6121 & 0.4551 & 0.6116 & 0.7509 & 0.5898 & 0.7247 & 0.7379 & 0.5708 & 0.7366 & 0.7165 & 0.5393 & 0.6949 \\
% \hline
% SVM & 0.6651 & 0.5031 & 0.6786 & 0.7418 & 0.5901 & 0.7321 & 0.7368 & 0.5866 & 0.7336 & 0.7265 & 0.5737 & 0.6964 \\
% \hline
% Random Forest & 0.614 & 0.4515 & 0.6592 & 0.7387 & 0.5502 & 0.7202 & 0.7317 & 0.5548 & 0.7173 & 0.7194 & 0.5636 & 0.7143 \\
% \hline
% \end{tabular}
% }
% \end{table*}
\MSI{Instead of creating subsubsections, we can briefly summarize the effects of removing lab-environment data.}
\subsubsection{Removing Lab-environment data from Test set}
In Table ~\ref{tab:res_super_park_not_in_test}, we present the results on Home-environment data by removing the  Lab-environment data from test set. As we are using leave-one-out-cross-validation, we have predictions on every data instance. We can see that the results exhibit almost the same pattern as in Table ~\ref{tab:res_with_super_park}. We are still getting the best performance using the Acoustic-features and the various models are performing almost the same. However, note that the test set of Table ~\ref{tab:res_with_super_park} and Table ~\ref{tab:res_super_park_not_in_training}  are not the same,hence the results are not directly comparable. But the results demonstrate that our models' performance do not get worse by excluding the Lab-environment data from test-set.

\subsection{Gender and age Stratified Analysis}

\subsubsection{Our Model's performance on Gender-stratified and age matched test-set}
\begin{table*}

 \caption{Group-Specific-Performance: These scores are achieved after training the model on entire dataset and then checking the performance of the model on three separate groups: Male, Female and Age-matched. Age-matched group is constructed from people over 50 years old. We can see that the performance for each sub-group is in par with the performance on the entire dataset (Table ~\ref{tab:res_with_super_park}), except for the Female group. This performance degradation can be attributed to the PD/Non-PD imbalance within the Female group (101 PD Vs. 300 Non-PD) }
  \label{tab:complete_model_gender_age_stratified}
\begin{tabular}{|l|l|l|l|l|l|l|}
\hline
Algorithm     & \multicolumn{2}{l|}{Male} & \multicolumn{2}{l|}{Female} & \multicolumn{2}{l|}{Age-matched} \\ \hline
              & AUC        & Accuracy     & AUC         & Accuracy      & AUC        & Accuracy    \\ \hline
SVM           & \textbf{0.7751}     & \textbf{0.7292}       & 0.6741      & 0.7556        & \textbf{0.7543}     & \textbf{0.7209}      \\ \hline
Random Forest & 0.7554     & 0.7262       & 0.6893      & 0.7606        & 0.7466     & 0.7209      \\ \hline
LightGBM      & 0.7461     & 0.6892       & \textbf{0.7238}      & \textbf{0.7456}        & 0.752      & 0.7039      \\ \hline
XGBoost       & 0.7549     & 0.72         & 0.7127      & 0.7581        & 0.7421     & 0.7225      \\ \hline
\end{tabular}
\end{table*}

We separately analyzed the performance of our models trained on Acoustic-features presented in Table ~\ref{tab:res_with_super_park} on three different data-sets: Male subjects, Female subjects and Age-matched subjects -- created by removing all subjects below the age of 50. The result is presented in Table ~\ref{tab:complete_model_gender_age_stratified}. We would like to reiterate that we did not train any model for this purpose. We just analyzed how our previous models are working on different population groups. 
% As we employed leave-one-out cross validation, each data-point is put in the test set once. Therefore, we have prediction for all data-points.

From Table ~\ref{tab:complete_model_gender_age_stratified}, we can see that the best model's in each of Male and Age-matched domains have similar or better performance to the overall model's mentioned in Table~\ref{tab:res_with_super_park} in terms of AUC. However, the model performs worse for Female subjects in comparison to all subjects. As we can see from the demographics information in Table. ~\ref{tab:demography}, females are over-represented in the Non-PD group and under-represented in the PD group. Previous Epidemiological studies have shown that both incidence and prevalence of PD are 1.5–2 times higher in men than in women~\cite{van2003incidence,haaxma2007gender}. Therefore, we are more likely to get PD data-samples from male than female. To improve our model's performance, we plan to include more female PD subjects in our dataset in future.
